# Supplementary material for: Deep Identification of Propagation Trees
Source: arXiv:2503.00646 source file (2025-03-01)
Supplement: Supplementary file 1 [file appendix.tex]

% \section{Dataset Description}
% We conduct experiments on five real-world datasets, with their basic statistics presented in Table~\ref{tab:datasets}:
% \begin{itemize}
%     \item \textbf{Cora-ML}~\cite{cora}: A citation network of computer science research papers, where nodes represent papers and edges indicate citation relationships.
%     \item \textbf{Power Grid}~\cite{powergrid}: The topology network of the Western States Power Grid of the US. Nodes represent generators, transformers, or substations, while edges correspond to power supply lines.
%     \item \textbf{Memetracker}~\cite{memetracker}: Tracks frequently appearing posts across the online news spectrum. Each story's propagation is recorded as a diffusion cascade.
% \end{itemize}
% \section{Additional Visualizations}

% \begin{table}[h]
%     \centering
%     \caption{Basic statistics of the datasets.}
%     \label{tab:datasets}
%     \begin{tabular}{lccc}
%         \toprule
%         Dataset & Nodes & Edges & Type \\
%         \midrule
%         Cora-ML & XX & XX & Citation \\
%         Power Grid & XX & XX & Infrastructure \\
%         Power Grid & XX & XX & Infrastructure \\
%         Memetracker & XX & XX & News Propagation \\
%         \bottomrule
%     \end{tabular}
% \end{table}
